# Supplementary material for: Steepest Descent Neural Architecture Optimization: Escaping Local Optimum with Signed Neural Splitting
Source: arXiv:2003.10392 source file (2021-06-21)
Supplement: Supplementary file 1 [file appendix_classification.tex]

\subsection{Convergence Rate for Classification Loss}

Now we generalize the theorem to classification case. For simplicity, we consider the binary classification problem with label $y\in\{0,1\}$. The (cross-entropy) training loss is defined as 
\[
\ell(\th)=-\frac{1}{n}\sum_{i=1}^{n}\left[y^{(i)}\log\left(p(f_{\th}(x))\right)+(1-y^{(i)})\log\left(1-p(f_{\th}(x))\right)\right],
\]
where
\[
p(f_{\th}(x))=\frac{\exp(f_{\th}(x^{(i)}))}{1+\exp(f_{\th}(x^{(i)}))}.
\]
And define the likelihood function 
\[
\frac{1}{n}\sum_{i=1}^{n}p(\th\mid x^{(i)},y^{(i)})=\frac{1}{n}\sum_{i=1}^{n}\left(p(f_{\th}(x))y^{(i)}+(1-p(f_{\th}(x)))(1-y^{(i)})\right).
\]
Notice that the likelihood function is no greater than 1.
\begin{lem} \label{lem:globalopt_class}
Under the same assumptions of Lemma \ref{lem:globalopt}, for any $\theta_{j}$, if $\left|\lambda_{\max}\left(\S(\theta_{j})\right)\right|\lor\left|\lambda_{\min}\left(\S(\theta_{j})\right)\right|\le\epsilon,$ we have 
\[
\frac{1}{n}\sum_{i=1}^{n}p(\th\mid x^{(i)},y^{(i)})\ge1-\sqrt{\frac{nh^{2}d\epsilon^{2}}{a_{j}^{4}\lambda}}.
\]
\end{lem}
Similarly, we are able to maximize the likelihood with arbitrarily accuracy.

\subsection{Proof of Lemma \ref{lem:globalopt_class}}
Simple algebra shows that the splitting matrix of neuron $\theta_{j}$
is 
\[
\S(\theta_{j})=\frac{\alpha_{j}^{2}}{n}\sum_{i=1}^{n}e_{i}(\theta)\sigma''(\theta_{j}^{\top}x^{(i)})x^{(i)}x^{(i)\top},
\]
where 
\[
e_{i}(\th)=\frac{-y^{(i)}+(1-y^{(i)})\exp(f_{\th}(x^{(i)}))}{1+\exp(f_{\th}(x^{(i)}))}.
\]
 Also notice that
\[
1-\frac{1}{n}\sum_{i=1}^{n}e_{i}(\th)=\frac{1}{n}\sum_{i=1}^{n}p(\th\mid x^{(i)},y^{(i)}).
\]
Using the same argument, we know that 
\[
\sqrt{\frac{1}{n}\sum_{i=1}^{n}e_{i}^{2}(\th)}\le\sqrt{\frac{nh^{2}d\epsilon^{2}}{a_{j}^{4}\lambda}}.
\]
Also notice that 
\[
\frac{1}{n}\sum_{i=1}^{n}e_{i}(\th)\le\frac{1}{n}\sum_{i=1}^{n}\left|e_{i}(\th)\right|\le\sqrt{\frac{1}{n}\sum_{i=1}^{n}e_{i}^{2}(\th)}.
\]
Thus we have $\frac{1}{n}\sum_{i=1}^{n}p(\th\mid x^{(i)},y^{(i)})\ge1-\sqrt{\frac{nh^{2}d\epsilon^{2}}{a_{j}^{4}\lambda}}$.

\begin{thm} \label{thm:main2}
For the classification case, under the same assumptions of theorem \ref{thm:main}, we are able to obtain a neural network with 
$
\frac{1}{n}\sum_{i=1}^{n}p(\th\mid x^{(i)},y^{(i)})\ge1-\epsilon,
$
and with $\mathcal{O}\left(\sqrt{\frac{nd}{\lambda}}h\epsilon^{-\frac{7}{6}}\right)+m$ neurons.
\end{thm}
