# Supplementary material for: Steepest Descent Neural Architecture Optimization: Escaping Local Optimum with Signed Neural Splitting
Source: arXiv:2003.10392 source file (2021-06-21)
Supplement: Supplementary file 3 [file bak_appendix_old_spliting3.tex]

\subsection{Derivation of Triplet Splittings ($m=3$)}

%\red{[We need to prove the case when $S$ does not $d$ distinctive eigen-values]. }

\begin{thm}
 Consider the optimization in \eqref{equ:optIIneg} with $m =3$ and $c\geq 1$. 
 Assume $S(\theta) \in \RR^{d\times d}$ has $d$ distinctive eigen-values, that is, there are no two eigen-vectors who share the same eigen-values. 
 
1)  The optimal solution must satisfy 
$$\delta_i = \sum_{\ell=1}^{d_r}r_{i,\ell} v_\ell, 
$$
where $\{v_\ell\}_{i=1}^{d_r}$  is a set of orthonormal eigen-vectors of $S(\theta)$ that share the same eigenvalue $\lambda$, 
and $\{r_{i,\ell}\}_{i,\ell}$ is a set of coefficients. 
%and $r_1, r_2, r_3 \in \R$ are three scalars. 

2) In this case, the optimization in \eqref{equ:optIIneg} is equivalent to 
\begin{align} \label{equ:R3Opt}
\begin{split} 
    G_3^{-c}:= 
    %\min_{w_1,w_2,r_1,r_2}  
    \min_{\vv w, \vvr, v} 
     (w_1 r_1^2 & + w_2 r_2^2 + w_3 r_3^2)\times  (v^\top S(\theta) v)  \\ %\lambda \\  ~~~~%\\ %\lambda_i  \\
    s.t. ~~~&  w_1 + w_2 + w_3 = 1 \\
    & w_1 r_1 + w_2 r_2 + w_3 r_3  = 0 \\
    & |w_1| + |w_2|   + |w_3|\leq c \\
    & |r_1|, |r_2| , |r_3|\leq 1 \\
    & \norm{v} \leq 1, ~~~ v\in \RR^d.
    \end{split}
    \end{align}
    
3)    % Therefore, we have 
The optimal value above is 
%In this casewe have 
\begin{align}\label{equ:G2capp}
G_{3}^{-c} = 
\min\left (  \frac{c+1}{2}\lambdamin, ~~  -\frac{c-1}{2} \lambdamax , ~~
0 \right ). 
%\min(R_2^{\min}\lambda_{\min}, ~~ R_2^{\max}\lambda_{\max}) ,
\end{align}
%where $R_2^\min$ and $R_2^\max$ are defined by \eqref{equ:R2min} and \eqref{equ:R2max}, respectively.  
If $-\frac{c-1}{2} \lambda_{\max} <  \frac{c+1}{2}\min(\lambdamin,0)$, the optimal solution is achieved by 
\begin{align*} 
        \left (w_1 = - \frac{c-1}{4}, ~~~~ \delta_1 =v_{\max}\right), &&  
         \left (w_2 = - \frac{c-1}{4}, ~~~~ \delta_2 =  - v_{\max} \right), &&
         \left (w_3 = \frac{c+1}{2}, ~~~~ \delta_3 = 0 \right).          
        \end{align*}
If $
\frac{c+1}{2}\lambda_{\min} <  
-\frac{c-1}{2}\max(\lambdamax,0)$ 
%\geq \lambda_{\min}$ 
%$G_2^{-c} = \lambda_{\min}$, 
the optimal solution is achieved by 
\begin{align*} 
        \left (w_1 =  \frac{c+1}{4}, ~~~~ \delta_1 =v_{\min}\right), &&  
         \left (w_2 =  \frac{c+1}{4}, ~~~~ \delta_2 =  - v_{\min} \right), &&
         \left (w_3 = -\frac{c-1}{2}, ~~~~ \delta_3 = 0 \right).          
        \end{align*}
If $0\leq \min\left( \frac{c+1}{2}\lambdamin, ~-\frac{c-1}{2} \lambdamax \right)$, and hence 
$\lambdamin =\lambdamax = 0$, the optimal solution is achieved by no splitting: $\delta_1=\delta_2=\delta_3=0$.         
\end{thm} 
%ÇﬁIf $\lambda_{\min} = \lambda_{\max}$
\begin{proof}
%Due to $w$
%By the constraint of
1) 
Note that we have by the constraint that $w_1 \delta_1 + w_2 \delta_2 + w_3 \delta_3 = 0$ and $\delta_1, \delta_2, \delta_3$ must be eigen-vectors of $S(\theta)$ following Lemma~\ref{lem:eigen}. 
By the assumption, all the eigen-vectors of $S(\theta)$ 
are linearly independent with each other. This suggests that all $\delta_i$ should be parallel to an eigen-vector $v$, that is, 
$\delta_i = r_i v$ for $i=1,2,3$. 


\red{TODO:} 
Following Lemma~\ref{lem:eigen}, the optimal $\delta_1,\delta_2, \delta_3$ are eigen-vectors of $S(\theta)$. 
Because eigen-vectors associated with different eigen-values are linearly independent, we can see that  
$\delta_1,\delta_2, \delta_3$ must share the same eigen-value due to the constraint  $w_1 \delta_1 + w_2 \delta_2 + w_3 \delta_3 =0$. If each eigen-value of $S(\theta)$ has only one eigen-direction, then we already prove the result. 
Otherwise, assume the optimal solution has  a form of  $\delta_i = \sum_{\ell} r_{i,\ell} v_\ell$ for $i=1,2,3$, where $\{v_\ell\}_\ell$ is a set of orthogonal  unit eigen-vectors of $S(\theta)$ shared with the same eigen-value $\lambda$, and $r_{i,\ell}$ the coefficient of $\delta_i$ on $v_\ell$. Then we have the optimization problem reduces to 
%%
\begin{align} %\label{equ:R3Opt}
\begin{split} 
    %G_3^{-c}:= 
    %\min_{w_1,w_2,r_1,r_2}  
    \min_{\vv w, \vvr, v} 
     \sum_{\ell}(w_1 r_{1,\ell}^2 & + w_2 r_{2,\ell}^2 + w_3 r_{3,\ell}^2)\times  \lambda \\ %\lambda \\  ~~~~%\\ %\lambda_i  \\
    s.t. ~~~&  w_1 + w_2 + w_3 = 1 \\
        & |w_1| + |w_2|   + |w_3|\leq c \\
    & w_1 r_{1,\ell} + w_2 r_{2,\ell} + w_3 r_{3,\ell}  = 0,~~~\forall \ell \\
    & \sum_{\ell} r_{i,\ell}^2\leq 1,~~~\forall \ell \\
    &  S(\theta) v_\ell = \lambda v_\ell,~~~\forall \ell.
    %\norm{v} \leq 1, ~~~ v\in \RR^d.
    \end{split}
    \end{align}
    
\begin{align}% \label{}
\begin{split} 
    %G_3^{-c}:= 
    %\min_{w_1,w_2,r_1,r_2}  
    \min_{\vv w, \vvr} 
     %\sum_{\ell}
     (
     w_1 \norm{\vvr_{1}}^2 & + w_2 \norm{\vvr_{2}}^2 + w_3 \norm{\vvr_{3}}^2)\times  \lambda \\ %\lambda \\  ~~~~%\\ %\lambda_i  \\
    s.t. ~~~&  w_1 + w_2 + w_3 = 1 \\
        & |w_1| + |w_2|   + |w_3|\leq c \\
    & w_1 \vvr_{1} + w_2 \vvr_{2} + w_3 \vvr_{3}  = 0,~~~\forall \ell \\
    & \norm{\vvr_{i}} \leq  1 ~~~\forall i=1,2,3.
    %&  S(\theta) v_\ell = \lambda v_\ell,~~~\forall \ell.
    %\norm{v} \leq 1, ~~~ v\in \RR^d.
    \end{split}
    \end{align}    
Without loss of generality, assume $r_{1,1}\leq 1$ and $r_{1,\ell}=0$ for $\ell\geq 2$. Then the optimization w.r.t. $(r_{2,\ell}, r_{3,\ell})$ for $\ell\geq 2$ reduces to 
\begin{align} %\label{equ:R3Opt}
\begin{split} 
    \min_{\vv w, \vvr, v} 
        (w_1 r_{1,1}^2  & +  w_2 r_{2,1}^2  +  w_3 r_{3,1}^2 )\times  \lambda +  
     \sum_{\ell\geq 2}( w_2 r_{2,\ell}^2 + w_3 r_{3,\ell}^2)\times  \lambda \\ %\lambda \\  ~~~~%\\ %\lambda_i  \\
    s.t. ~~~&  w_1 + w_2 + w_3 = 1 \\
        & |w_1| + |w_2|   + |w_3|\leq c \\
    &    w_1 r_{1,1} +  w_2 r_{2,1}  +  w_3 r_{3,1} =0\\
    &  w_2 r_{2,\ell} + w_3 r_{3,\ell}  = 0,~~~\forall \ell\geq 2 \\
    & |r_{1,1}|  \leq 1 \\
    & \sum_{\ell} r_{2,\ell}^2\leq 1\\
    & \sum_{\ell} r_{3,\ell}^2\leq 1\\
    &  S(\theta) v_\ell = \lambda v_\ell,~~~\forall \ell.
    %\norm{v} \leq 1, ~~~ v\in \RR^d.
    \end{split}
    \end{align}
    Assume $r_{2,\ell} = w_3 \alpha_\ell$ and $r_{3,\ell} = -w_2 \alpha_\ell$, we have 
\begin{align} %\label{equ:R3Opt}
\begin{split} 
    \min_{\vv w, \vvr, v} 
    (w_1 r_{1,1}^2  & +  w_2 r_{2,1}^2  +  w_3 r_{3,1}^2 )\times  \lambda + 
     \sum_{\ell\geq 2} w_2 w_3  (w_2+ w_3)\alpha_{\ell}^2\times  \lambda \\ %\lambda \\  ~~~~%\\ %\lambda_i  \\
    s.t. ~~~&  w_1 + w_2 + w_3 = 1 \\
        & |w_1| + |w_2|   + |w_3|\leq c \\
    &    w_1 r_{1,1} +  w_2 r_{2,1}  +  w_3 r_{3,1} =0\\
    %&  w_2 r_{2,\ell} + w_3 r_{3,\ell}  = 0,~~~\forall \ell\geq 2 \\
    & |r_{1,1}|  \leq 1 \\
    & r_{2,1}^2 +  w_3^2\sum_{\ell\geq 2} \alpha_{\ell}^2\leq 1 \\ %%,
    & r_{3,1}^2 + w_2^2\sum_{\ell\geq 2} \alpha_{\ell}^2\leq 1 \\ %%, ~~~\forall i \\
%    ~~~\forall i \\
    &  S(\theta) v_\ell = \lambda v_\ell,~~~\forall \ell.
    %\norm{v} \leq 1, ~~~ v\in \RR^d.
    \end{split}
    \end{align}    
Let $\alpha^2 :=\sum_{\ell\geq 2}\alpha_\ell^2$, we have 
\begin{align} %\label{equ:R3Opt}
\begin{split} 
    \min_{\vv w, \vvr, v} 
    (w_1 r_{1,1}^2  & +  w_2 r_{2,1}^2  +  w_3 r_{3,1}^2 )\times  \lambda + 
 w_2 w_3  (w_2+ w_3)\alpha^2 \times  \lambda \\ %\lambda \\  ~~~~%\\ %\lambda_i  \\
    s.t. ~~~&  w_1 + w_2 + w_3 = 1 \\
        & |w_1| + |w_2|   + |w_3|\leq c \\
    &    w_1 r_{1,1} +  w_2 r_{2,1}  +  w_3 r_{3,1} =0\\
    %&  w_2 r_{2,\ell} + w_3 r_{3,\ell}  = 0,~~~\forall \ell\geq 2 \\
    & |r_{1,1}|  \leq 1 \\
    & r_{2,1}^2 +  w_3^2\alpha^2\leq 1 \\ %%,
    & r_{3,1}^2 + w_2^2\alpha^2\leq 1 \\%    & %w_3^2\sum_{\ell\geq 2} \alpha_{\ell}^2\leq 1 \\ %%, ~~~\forall i \\
%    ~~~\forall i \\
    &  S(\theta) v_\ell = \lambda v_\ell,~~~\forall \ell.
    %\norm{v} \leq 1, ~~~ v\in \RR^d.
    \end{split}
    \end{align}    
2) Plugging $\delta_i= r_iv$, $i=1,2,3$ into \eqref{equ:optIIneg} directly implies \eqref{equ:R2Opt}. 

3) 
Following Lemma~\ref{lem:solve3min} and \ref{lem:solve3max},  
the value of $w_1 r_1^2 + w_2 r_2^2 + w_3 r_3^2$ in \eqref{equ:R3Opt} can range from $-\frac{c-1}{2}$ to $\frac{c+1}{2}$. 
In addition, the range of $\{ v^\top S(\theta) v \colon ~~ \norm{v}\leq 1 \}$ is $[ \min(\lambdamin,0), \max(\lambdamax,0)]$.  
Therefore, we can write 
\begin{align*}
G_2^{-c}  
& = \min_{t, v}\left \{ t \times \lambda \colon ~~~ -\frac{c-1}{2} \leq t \leq \frac{c+1}{2}, ~~~ \min(\lambdamin,0) \leq \lambda \leq  \max(\lambdamax,0) \right\} \\
& = \min\left (
-\frac{c-1}{2} \max(\lambdamax,0), ~~~
\frac{c+1}{2} \min(\lambdamin,0)
\right). 
%G_2^{-c}  = \min_{t, v}\left \{ t \times (v^\top S(\theta) v) \colon ~~~ -\frac{c-1}{c+1} \leq t \leq 1, ~~~ \norm{v}\leq 1 \right\}. 
\end{align*}
This implies the result in \eqref{equ:G2capp}. The corresponding optimal solutions follow Lemma~\ref{lem:solve3min} and \ref{lem:solve3max}. 
%$\delta_1$ and 
%the solution must have 
\end{proof}


\begin{lem}\label{lem:solve3min}
For $c \geq 1$, consider the following optimization: 
\begin{align*}
    R_3^{\min}:= \min_{(\vv w, \vvr)\in \RR^6}   
%    F(\vv w, \vvr) := 
     w_1 r_1^2 + & w_2 r_2^2 + w_3 r_3^2 \\  ~~~~%\\ %\lambda_i  \\
    s.t. ~~~&  w_1 + w_2 + w_3  = 1 \\
    & w_1 r_1 + w_2 r_2 + w_3 r_3 = 0 \\
    & |w_1| + |w_2| + |w_3| \leq c \\
    & |r_1|, |r_2|, |r_3|\leq 1.
    \end{align*}
    We have $R_3^{\min} = - \frac{c-1}{2}$, and this is achieved by 
    the following solution 
        \begin{align}\label{equ:3spliting1app}
         \left (w_1 =  - \frac{c-1}{4},~~~~ r_1 =1 \right), &&
         \left (w_2 = - \frac{c-1}{4},~~~~ r_2 = -1 \right), &&
         \left (w_3 = \frac{c+1}{2}, ~~~~ r_3 =0 \right).  
    \end{align}
    %which yields $F^*_{min} = -\frac{c-1}{2}$. 
\end{lem}
\begin{proof}
%Case $$
%
\noindent\textbf{Case 1 (two negative weights, one positive weight)}~~ Without loss of generality, we assume $w_1<0$, $w_2 < 0$, $w_3>1$. 
For notation, let $w_1 = -a_1 < 0$, $w_2 = -a_2<0$ and hence $w_3 = 1-w_1 - w_2 = 1+a_1 + a_2$.
Because $w_1r_1^2 + w_2 r_2^2 + w_3r^2$ is a concave function of $(r_1,r_2)$ in this case, the optimal solution must be achieved by either $|r_1| =1$ or $|r_2| =1$; see also Lemma~\ref{lem:r1r2neg}. Without loss of generality, we can assume $r_1 =1$. In this case, the optimization reduces to 
\begin{align*}
    %F^*_{min}:= 
    \min_{a_1,a_2, r_2,r_3}  
     -a_1  - a_2 r_2^2 & + (1+a_1 + a_2) r_3^2 \\
     ~~~~s.t.~~~~%\\ %\lambda_i  \\
    %s.t. ~~~&  w_1 + w_2 + w_3  = 1 \\
    & a_1  + a_2 r_2 =(1+a_1+a_2) r_3 \\
    &  a_1 \geq 0, a_2 \geq 0, ~ 1+2(a_1+a_2) \leq c \\
    %|w_1| + |w_2| + |w_3| \leq c \\
    &  |r_2|\leq 1, ~~|r_3|\leq 1.
    \end{align*}
%$Canceling
Writing $\eta = w_3 r_3 = (1+a_1+a_2) r_3$ and eliminating $r_2$, 
then $|r_3|\leq 1$ is equivalent to $|\eta|\leq 1+a_1 + a_2$ and $|r_2|\leq 1$ is equivalent to $ |\eta - a_1| \leq a_2$. We get 
\begin{align}\label{equ:aropt}
    %F^*_{min}:= 
    \min_{a_1, a_2,\eta} 
      -a_1  -& \frac{(\eta -  a_1)^2}{a_2} + \frac{\eta^2}{1+a_1+a_2} \\
     ~~~~s.t.~~~~%\\ %\lambda_i  \\
    %s.t. ~~~&  w_1 + w_2 + w_3  = 1 \\
    %& w_1  + w_2 r_2 + w_3 r_3 = 0 \\
    &  a_1 \geq 0, ~~~a_2 \geq 0 \\
    & 1+2(a_1+a_2) \leq c \\
    %|w_1| + |w_2| + |w_3| \leq c \\
    &  |\eta|\leq 1+a_1 + a_2\\
    & |\eta - a_1| \leq a_2.
    \end{align}
    Because 
    $|\eta - a_1| \leq a_2$  implies $|\eta|\leq a_1 + a_2 \leq 1+ a_1 + a_2$, the constraint $|\eta| \leq 1+a_1+a_2$ is always inactive and hence can be dropped.  
    Therefore, the optimization  reduces to 
    $$
    \min_{\eta, a_1, a_2} -a_1  - \frac{(\eta -  a_1)^2}{a_2} + \frac{\eta^2}{1+a_1+a_2}~~~~s.t.~~~~~ a_1 - a_2 \leq \eta \leq a_1 + a_2, ~~~  a_1 \geq 0, ~~~a_2 \geq 0, ~ a_1+a_2\leq \frac{c-1}{2}.
    $$
    Considering the optimization w.r.t. $\eta$, we note that it is a  minimization of  %This minimizes 
    a concave quadratic function (because the leading term $(-\frac{1}{a_2}+\frac{1}{1+a_1+a_2})\eta^2$ is negative). 
    Therefore, the optimal $\eta$ is achieved on the vertex of the constraint set, either $\eta = a_1 - a_2$ or $\eta = a_1+ a_2$. A simple calculation shows that $\eta = a_1 - a_2$ is always a better solution. 
    
    Plugging $\eta = a_1 - a_2$, the optimization further reduces to 
    \begin{align*}%\label{equ:aropt}
    \min_{a_1, a_2}  
     -a_1  - a_2 + \frac{(a_1 - a_2)^2}{1+a_1 + a_2} 
     ~~~~s.t.~~~~%\\ %\lambda_i  \\
    %s.t. ~~~&  w_1 + w_2 + w_3  = 1 \\
    %& w_1  + w_2 r_2 + w_3 r_3 = 0 \\
    a_1 \geq 0,~~~ a_2 \geq 0, ~~~~
      a_1+a_2\leq \frac{c-1}{2}. 
    \end{align*}
    It is easy to see that the optimal solution is achieved when $a_1 = a_2 = \frac{c-1}{4}$, which implies that $\eta = a_1 - a_2 = 0$.  
    This corresponds to the solution in \eqref{equ:3spliting1app}, 
    and it is easy to verify that it achieves an optimal value of $-\frac{c-1}{2}$. 
%    To summarize, in this case we have 
    %\begin{align*}
        %& w_1 = w_2 = - \frac{c-1}{4}, ~~~~ w_3 = \frac{c+1}{2} \\
        %& r_1 = 1, r_2 = -1 ~~~ r_3 = 0 \\
    %\end{align*}
    
    
\noindent\textbf{Case 2 (two positive weights, one negative weight)}~~
Without loss of generality, we can assume $w_1 >0$, $w_2 >0$, $w_3 < 0$. 
Taking $\eta = - w_3 r_3$, then we have $|\eta| \leq |w_3| = - w_3 = w_2 + w_1 - 1 < w_1+w_2$. 
Following Lemma~\ref{lem:r1r2} below, the optimal solution must satisfy $r_1 = r_2$  in this case.
This means that problem reduces to the case of $m=2$ in \eqref{equ:R2min}, which achieves an optimal value of $-\frac{c-1}{c+1}$. 
However, because $-\frac{c-1}{2} \leq -\frac{c-1}{c+1}$ when $c\geq 1$, this case is always subsumed by Case 1. 
%the splitting can be reduced to a binary splitting by combining $r_1$ and $r_2$. Therefore, the triplet splitting is not better than binary splitting in this case. 

\noindent \textbf{Case 3 (three positive weights)}~~
%We have $w_1\geq $
This case can never be the optimal solution because  $w_1 r_1^2 + w_2 r_2^2 + w_3 r_3^2\geq 0 \geq -\frac{c-1}{2}$.
    

Overall, the optimal solution is achieved by Case 1, which yields
$R_3^{\min}= -\frac{c-1}{2}$ and the optimal solution in \eqref{equ:3spliting1app}. 
\end{proof}



\begin{lem}\label{lem:solve3max} 
For $c \geq 1$, consider the following optimization: 
\begin{align*}
    R_3^{\max}:= \max_{(\vv w, \vvr)\in \RR^6}   
%    F(\vv w, \vvr) := 
     w_1 r_1^2 + & w_2 r_2^2 + w_3 r_3^2 \\  ~~~~%\\ %\lambda_i  \\
    s.t. ~~~&  w_1 + w_2 + w_3  = 1 \\
    & w_1 r_1 + w_2 r_2 + w_3 r_3 = 0 \\
    & |w_1| + |w_2| + |w_3| \leq c \\
    & |r_1|, |r_2|, |r_3|\leq 1.
    \end{align*}
    We have $R_3^{\max} =\frac{c+1}{2}$, and this is achieved by 
    the following solution 
\begin{align}\label{equ:3spliting1appneg} 
\left ( w_1 = \frac{c+1}{4},~~~
r_1 = 1
\right ) &&
\left ( w_2 = \frac{c+1}{4},~~~
r_2 = -1
\right ) &&
\left ( w_3 = -\frac{c-1}{2},~~~
r_3 = 0
\right ).
\end{align}
    %which yields $F^*_{min} = -\frac{c-1}{2}$. 
\end{lem}
\begin{proof}
%Case $$
%
\noindent\textbf{Case 1 (two negative weights, one positive weight)}~~ Without loss of generality, we assume $w_1<0$, $w_2 < 0$, $w_3>1$. 
For notation, let $w_1 = -a_1 < 0$, $w_2 = -a_2<0$ and hence $w_3 = 1-w_1 - w_2 = 1+a_1 + a_2$.  
Write $\eta = (1+a_1+a_2) r_3$. 
In this case, the optimization reduces to 
\begin{align*}
    %R_3^{\max}:= 
    \max_{a_1,a_2,r_1,r_2,\eta}   
%    F(\vv w, \vvr) := 
     -a_1 r_1^2 - & a_2 r_2^2 + 
     \frac{\eta^2}{1+a_1+a_2} \\%% r_3^2 \\  ~~~~%\\ %\lambda_i  \\
    s.t. ~~~%&  w_1 + w_2 + w_3  = 1 \\
    & a_1 r_1 + a_2 r_2 =\eta, ~~~|r_1|, |r_2| \leq 1 \\ 
    & a_1+a_2 \leq \frac{c-1}{2}, ~~~
%    & 
     |\eta|\leq 1+a_1 + a_2. 
    \end{align*}
Considering the optimization of $(r_1, r_2)$ with fixed $(a_1,a_2,\eta)$. There are two cases. 

Case 1.1. If the constraints $|r_1|, |r_2| \leq 1$ are inactive, the optimal solution must satisfy $r_1 = r_2$ (see Lemma~\ref{lem:r1r2}), and hence the optimization can be reduced to the case of binary splitting $(m=2)$ in \eqref{equ:R2max}. The optimal value achieved in this case equals $1$ following Lemma~\ref{lem:solve2max}. 

Case 1.2. If the constraint $|r_1|, |r_2| \leq 1$ are active, we assume $r_1 = 1$ without loss of generality. Then the optimization reduces to 
\begin{align*}
    %R_3^{\max}:= 
    \max_{a_1,a_2, r_2,\eta}   
%    F(\vv w, \vvr) := 
     -a_1  - & a_2 r_2^2 + 
     \frac{\eta^2}{1+a_1+a_2} \\%% r_3^2 \\  ~~~~%\\ %\lambda_i  \\
    s.t. ~~~%&  w_1 + w_2 + w_3  = 1 \\
        & a_1+a_2 \leq \frac{c-1}{2}, ~~~ a_1, a_2\geq 0\\
    & a_1  + a_2 r_2 =\eta, ~~~ |r_2| \leq 1 \\ 
%    & 
     & |\eta|\leq 1+a_1 + a_2. 
    \end{align*}
    Eliminating $r_2$ gives 
\begin{align}\label{equ:tmpgood}
\begin{split}
    \max_{a_1,a_2,\eta}   
%    F(\vv w, \vvr) := 
     -a_1  - & \frac{(\eta - a_1)^2}{a_2} + 
     \frac{\eta^2}{1+a_1+a_2} \\%% r_3^2 \\  ~~~~%\\ %\lambda_i  \\
    s.t. ~~~%&  w_1 + w_2 + w_3  = 1 \\
    & a_1+a_2 \leq \frac{c-1}{2}, ~~~ a_1, a_2 \geq 0\\
    & |\eta - a_1| \leq a_2 \\ 
%    & 
     & |\eta|\leq 1+a_1 + a_2. 
     \end{split}
    \end{align}    
     The constraint $\eta \leq 1+a_1 + a_2$ is always inactive because it is implied by $|\eta-a_1|\leq a_2$. Therefore, the optimization w.r.t. $\eta$ is % have
\begin{align*}
    \max_{\eta}   
    \left(\frac{1}{1+a_1+a_2}-\frac{1}{a_2}\right) \eta^2 + \frac{2a_1}{a_2} \eta     -  a_1 - \frac{a_1^2}{a_2}
%    F(\vv w, \vvr) := 
     %-a_1  - & \frac{(\eta - a_1)^2}{a_2} +\frac{\eta^2}{1+a_1+a_2} \\%% r_3^2 \\  ~~~~%\\ %\lambda_i  \\
    ~~~~s.t.~~~~%&  w_1 + w_2 + w_3  = 1 \\
    %& a_1+a_2 \leq \frac{c-1}{2}, ~~~ a_1, a_2 \geq 0\\
    & a_1 - a_2\leq \eta \leq a_1 +  a_2. 
%    & 
     %& |\eta|\leq 1+a_1 + a_2. 
    \end{align*} 
    Because $\frac{1}{1+a_1+a_2}-\frac{1}{a_2} < 0$, this maximizes a concave quadratic function in an interval. The unconstraint maximum point is  
$$
\eta^* := \frac{-a_1}{a_2 (\frac{1}{1+a_1+a_2}-\frac{1}{a_2})} = 
\frac{a_1(1+a_1 + a_2)}{  1 + a_1} = a_1 + \frac{a_1 a_2}{1+a_1}. 
%= a_1 - a_2 + \frac{a_1a_2 + a_2 + a_1a_2}{1+a_1}
%= a_1 + a_2 + \frac{-a_2}{1+a_1}
$$
It is easy to verify that $\eta^* \in [a_1 - a_2, ~ a_1+ a_2]$ and hence $\eta^*$ is indeed the optimal solution. 
Plugging it into \eqref{equ:tmpgood}, we get \begin{align*}%\label{equ:tmpgood}
\begin{split}
    \max_{(\vv w, \vvr)\in \RR^6}   
     -a_1  - & 
     \frac{(a_1a_2)^2}{a_2(1+a_1)^2} + 
     \frac{a_1^2 (1+a_1+a_2)}{(1+a_1)^2} \\
    s.t. ~~~
    & a_1+a_2 \leq \frac{c-1}{2}, ~~~ a_1, a_2 \geq 0.\\
     \end{split}
    \end{align*} 
    As shown in Lemma~\ref{lem:wawadudu} below, this can be simplified to, % (see ) 
\begin{align*} 
\begin{split}
    \max_{(\vv w, \vvr)\in \RR^6}
     \frac{-a_1}{1+a_1} 
~~~~    s.t. ~~~~
    & a_1+a_2 \leq \frac{c-1}{2}, ~~~ a_1, a_2 \geq 0.\\
     \end{split}
    \end{align*}
The optimum is achieved when $a_1 = 0$. This means that the solution reduces to a binary splitting, whose maximum value is hence again at most $1$ following Lemma~\ref{lem:solve2max}.    


\begin{lem} \label{lem:wawadudu}
$$
  -a_1  - 
     \frac{(a_1a_2)^2}{a_2(1+a_1)^2} + 
     \frac{a_1^2 (1+a_1+a_2)}{(1+a_1)^2} = \frac{-a_1}{1+a_1}. 
$$
\end{lem}
\begin{proof} 
\begin{align*}%\label{equ:tmpgood}
\begin{split}
 & -a_1  - 
     \frac{(a_1a_2)^2}{a_2(1+a_1)^2} + 
     \frac{a_1^2 (1+a_1+a_2)}{(1+a_1)^2} = \frac{-a_1}{1+a_1} \\
   & =  \frac{-a_1a_2 (1+a_1)^2-a_1^2a_2^2 +
    a_2a_1^2 (1+a_1+a_2)
    }{a_2 (1+a_1)^2} \\
   & =  \frac{-a_1a_2
\left [ (1+a_1)^2+ a_1a_2 - 
    a_1 (1+a_1+a_2) \right ]
    }{a_2 (1+a_1)^2} \\
   & =  \frac{-a_1a_2
\left [  1+2 a_1 + a_1^2+ a_1a_2 - 
    a_1 -a_1^2 -  a_1a_2 \right ]
    }{a_2 (1+a_1)^2} \\     
   & =  \frac{-a_1a_2
\left [  1+ a_1  \right ]
    }{a_2 (1+a_1)^2} \\   
   & =  \frac{-a_1
    }{1+a_1} \\      
     \end{split}
    \end{align*}   
\end{proof}
%In this case, we have 
%$a_0 \leq a_1+a_2$. 
%maximum point of o
    
\noindent\textbf{Case 2 (two positive weights, one negative weight)}~~
Without loss of generality, we can assume $w_1 >0$, $w_2 >0$, $w_3 < 0$, and hence
$$
|w_1| + |w_2| + |w_3| = 2(w_1 + w_2) -  1 \leq c.
$$
In this case, we have the following obvious upper bound 
$$
R_3^{-c} = \max (w_1 r_1^2 + w_2 r_1^2 + w_3 r_3^2) \leq w_1 + w_2 \leq \frac{ c +1}{2}. 
$$
On the other hand, the upper bound is achieved by 
\begin{align}\label{equ:3spliting1appneg} 
\left ( w_1 = \frac{c+1}{4},~~~
r_1 = 1
\right ) &&
\left ( w_2 = \frac{c+1}{4},~~~
r_2 = -1
\right ) &&
\left ( w_3 = -\frac{c-1}{2},~~~
r_3 = 0
\right ).
\end{align}

\iffalse 
Without loss of generality, we can assume $w_1 >0$, $w_2 >0$, $w_3 < 0$. 
Taking $\eta = - w_3 r_3 = (w_1+w_2 -1) r_3$. %, then we have $|\eta| \leq |w_3| = - w_3 = w_2 + w_1 - 1 < w_1+w_2$. 
The optimization reduces to 
\begin{align*}
    %R_3^{\max}:= 
    \max_{(\vv w, \vvr)\in \RR^6}   
%    F(\vv w, \vvr) := 
     w_1 r_1^2 + & w_2 r_2^2 -  \frac{\eta^2}{w_1 + w_2 - 1} \\  ~~~~%\\ %\lambda_i  \\
    s.t. ~~~%&  w_1 + w_2 + w_3  = 1 \\
    & w_1 r_1 + w_2 r_2 = \eta  \\
    &  1 \leq w_1 + w_2 \leq \frac{c+1}{2}, ~~~~
    w_1, w_2 \geq 0  \\
    & |r_1|, |r_2|\leq 1,~~~~|\eta|\leq w_1+w_2 -1 
    \end{align*}

Following Lemma~\ref{lem:r1r2neg}, the optimal solution satisfies either $|r_1| =1$ or $|r_2| =1$. Without loss of generality, we can assume $r_1 =1$. In this case, the optimization reduces to 
\begin{align*}
    \max_{(\vv w, \vvr)\in \RR^6}   
%    F(\vv w, \vvr) := 
     w_1 + & w_2 r_2^2 -  \frac{\eta^2}{w_1 + w_2 - 1} \\  ~~~~%\\ %\lambda_i  \\
    s.t. ~~~%&  w_1 + w_2 + w_3  = 1 \\
    & w_1  + w_2 r_2 = \eta  \\
    &  1 \leq w_1 + w_2 \leq \frac{c+1}{2}, ~~~~
    w_1, w_2 \geq 0  \\
    & |r_2|\leq 1,~~~~|\eta|\leq w_1+w_2 -1 
    \end{align*}
%$Canceling
%Denoting by $\eta = w_3 r_3 = (1+a_1+a_2) r_3$ and 
Eliminating $r_2$, we get 
\begin{align*}
    \max_{(\vv w, \vvr)\in \RR^6}   
%    F(\vv w, \vvr) := 
     w_1 + &  \frac{(\eta - w_1)^2}{w_2} -  \frac{\eta^2}{w_1 + w_2 - 1} \\  ~~~~%\\ %\lambda_i  \\
    s.t. ~~~%&  w_1 + w_2 + w_3  = 1 \\
    %& w_1  + w_2 r_2 = \eta  \\
    &  1 \leq w_1 + w_2 \leq \frac{c+1}{2}, ~~~~
    w_1, w_2 \geq 0  \\
    & |\eta - w_1|\leq w_2,~~~~|\eta|\leq w_1+w_2 -1 
    \end{align*}
    The optimization of $\eta$ (with fixed $w_1, w_2$) can be re-framed to  
    \iffalse 
\begin{align*}
    \max_{\eta}    
     w_1 + &  \frac{(\eta - w_1)^2}{w_2} -  \frac{\eta^2}{w_1 + w_2 - 1} ~~~~~ ~~~~
    s.t. ~~~
    &    w_1 - w_2\leq  \eta \leq w_1 + w_2 - 1
    \end{align*}
    \fi
\begin{align*}
    \max_{\eta}
    \left ( \frac{1}{w_2} - \frac{1}{w_1+w_2 - 1} \right) \eta^2 - \frac{2w_1}{w_2} \eta + w_1 + \frac{w_1^2}{w_2}
     %w_1 + &  \frac{(\eta - w_1)^2}{w_2} -  \frac{\eta^2}{w_1 + w_2 - 1} 
     ~~~~~ ~~~~
    s.t. ~~~
    &    w_1 - w_2\leq  \eta \leq w_1 + w_2 - 1. 
    \end{align*}      
%    
    There are two cases: 
    
Case 2.1. 
If $w_1 \geq 1$, the solution is achieved on the vertex, either $\eta = w_1 - w_2$ and $\eta = w_1 + w_2 -1$. 

\begin{align*} 
& w_1 + w_2 - \frac{(w_1 - w_2)^2}{w_1 + w_2  -1} \\
& = \frac{(w_1 + w_2)(w_1 + w_2  -1)  - (w_1 - w_2)^2}{w_1 + w_2  -1} \\
& = \frac{ 4 w_1 w_2 - w_1 - w_2}{w_1 + w_2  -1} \\
& = - 1 + \frac{ 4 w_1 w_2 - 1}{w_1 + w_2  -1}
 \end{align*}
    
\begin{align*} 
& w_1 + \frac{(w_2 -1)^2}{w_2} 
- w_1 - w_2 + 1  \\
& =  \frac{(w_2 -1)^2}{w_2} 
 - w_2 + 1 \\
 & = \frac{(w_2 -1)^2 - w_2^2 + w_2}{w_2} \\
 & = \frac{- w_2 + 1}{w_2} \\
 & = -1 + \frac{1}{w_2}
\end{align*}
    
    %We must have $w_2 \geq  1/2\geq -w_2$
%If $w_1$
    
  
 
 
    Therefore, the optimization w.r.t. $\eta$ reduces to 
    $$
    \min_{\eta, a_1, a_2} -a_1  - \frac{(\eta -  a_1)^2}{a_2} + \frac{\eta^2}{w_3}~~~~s.t.~~~~~ a_1 - a_2 \leq \eta \leq a_1 + a_2, ~~~  a_1 \geq 0, ~~~a_2 \geq 0, ~ a_1+a_2\leq (c-1)/2.
    $$
    Considering the optimization w.r.t. $\eta$, we note that it is an minimization of  %This minimizes 
    a concave quadratic function (because the leading term $(-\frac{1}{a_2}+\frac{1}{1+a_1+a_2})\eta^2$ is negative). 
    Therefore, the optimal $\eta$ is achieved on the vertex of the constraint set, either $\eta = a_1 - a_2$ or $\eta = a_1+ a_2$. A simple calculation shows that $\eta = a_1 - a_2$ is always better solution. 
    
    Plugging $\eta = a_1 - a_2$, the optimization further reduces to 
    \begin{align*}%\label{equ:aropt}
    \min_{a_1, a_2}  
     -a_1  - a_2 + \frac{(a_1 - a_2)^2}{1+a_1 + a_2} 
     ~~~~s.t.~~~~%\\ %\lambda_i  \\
    %s.t. ~~~&  w_1 + w_2 + w_3  = 1 \\
    %& w_1  + w_2 r_2 + w_3 r_3 = 0 \\
    a_1 \geq 0,~~~ a_2 \geq 0, ~~~~
      a_1+a_2\leq \frac{c-1}{2}
    \end{align*}
    It is easy to see that the optimal solution is achieved when $a_1 = a_2 = \frac{c-1}{4}$, which implies that $\eta = a_1 - a_2 = 0$.  
    This corresponds to the solution in \eqref{equ:3spliting1app}, 
    and it is easy to verify that it achieves an optimal value of $-\frac{c-1}{2}$. 
%    To summarize, in this case we have 
    %\begin{align*}
        %& w_1 = w_2 = - \frac{c-1}{4}, ~~~~ w_3 = \frac{c+1}{2} \\
        %& r_1 = 1, r_2 = -1 ~~~ r_3 = 0 \\
    %\end{align*}
\fi     

\noindent \textbf{Case 3 (three positive weights)}~~
%We have $w_1\geq $
This case is always subsumed by Case 2, because when $w_1,w_2,w_3\geq 0$, we have $w_1 r_1^2 + w_2 r_2^2 + w_3 r_3^2\leq 1 \leq \frac{c+1}{2}$. 
%\geq -\frac{c-1}{2}$.
    
Overall, the optimal solution is achieved by Case 2, which yields
$R_3^{\max}= \frac{c+1}{2}$ and the optimal solution in \eqref{equ:3spliting1appneg}. 
\end{proof}

\begin{lem}\label{lem:r1r2}
Assume $w_1 > 0$, $w_2 >0$. 
If $|\eta| < w_1 + w_2$, then the optimal solution of 
\begin{align*}
&\min_{r_1, r_2} w_1 r_1^2 + w_2 r_2 ^2   ~~~s.t.~~~
&{w_1} r_1 + {w_2} r_2 = \eta,~~~~
|r_1| \leq 1, ~~ |r_2|\leq 1 %, ~~~ |\eta |\leq t. 
\end{align*} 
is achieved by $\displaystyle r_1 = r_2  = \frac{\eta}{w_1+ w_2}$.
\end{lem}
\begin{proof}
Canceling out $r_2$, we have 
$$
w_1 r_1^2 + w_2 r_2 ^2  = w_1 w_2 r_1^2 + (\eta - w_1 r_1)^2
= w_1 (w_1+w_2) r_1^2 - 2\eta w_1 r_1 + \eta^2.
$$
It is minimum is achieved by $r_1 = \eta/(w_1+ w_2)$ and consequently, $r_2 = \eta /(w_1 +w_2)$. Because $|\eta| \leq w_1+w_2$, the condition that $|r_1| \leq 1$ and $|r_2 |\leq 1$ is satisfied. This shows the optimization is solved. 
\end{proof}

\begin{lem}\label{lem:r1r2neg}
Assume $w_1 < 0$, $w_2 < 0$, %If $|\eta| < w_1 + w_2$, 
then the optimal solution of 
\begin{align*}
&\min_{r_1, r_2} w_1 r_1^2 + w_2 r_2 ^2   ~~~s.t.~~~
&{w_1} r_1 + {w_2} r_2 = \eta,~~~~
|r_1| \leq 1, ~~ |r_2|\leq 1 %, ~~~ |\eta |\leq t. 
\end{align*} 
must satisfy either $|r_1| = 1$ or $|r_2| = 1$. 
\end{lem}
\begin{proof}
This is because we are minimizing a concave function, and hence the optimal solution must lie on one of the vertexes of the constraint set. 
\end{proof}




\iffalse 
\subsection{A simpler proof for Triplet Splittings}

\paragraph{Case 1 $\protect\w_{1}\ge0$, $\protect\w_{2}\le0$, $\protect\w_{3}\le0$}

We further assume that $\delta_{1}=\alpha\delta_{\max}$, $\delta_{2}=\beta\delta_{\max}$
and $\delta_{3}=\gamma\delta_{\max}$. And thus our constraint optimization
convert to 
\begin{align*}
\min_{\d,\boldsymbol{\w}} & \ \w_{1}\alpha^{2}+\w_{2}\beta^{2}+\w_{3}\gamma^{2}\\
\text{s.t.} & \ \w_{1}\alpha+\w_{2}\beta+\w_{3}\gamma=0\\
 & \ \sum_{i=1}^{m}\w_{i}=1\\
 & \ \left|\alpha\right|,\left|\beta\right|,\left|\gamma\right|\le1\\
 & \ \sum_{i=1}^{m}\left|\w_{i}\right|\le c.
\end{align*}
By letting $\w_{4}=\w_{2}+\w_{3}\le0$, the problem reduces to 
\begin{align*}
\min_{\d,\boldsymbol{\w}} & \ \w_{1}\alpha^{2}+\left(\beta^{2}+\gamma^{2}\right)\w_{4}\\
\text{s.t.} & \ \w_{1}\alpha+\left(\beta+\gamma\right)\w_{4}=0\\
 & \ \w_{1}+\w_{4}=1\\
 & \ \left|\alpha\right|,\left|\beta\right|,\left|\gamma\right|\le1\\
 & \ \left|\w_{1}\right|+\left|\w_{4}\right|\le c.
\end{align*}
This is equivalent to
\begin{align*}
\min_{\d,\boldsymbol{\w}} & \ \left[-\left(\beta+\gamma\right)\alpha+\left(\beta^{2}+\gamma^{2}\right)\right]\w_{4}\\
\text{s.t.} & \ (1-\w_{4})\alpha+\left(\beta+\gamma\right)\w_{4}=0\\
 & \ \left|\alpha\right|,\left|\beta\right|,\left|\gamma\right|\le1\\
 & \ \frac{1-c}{2}\le\w_{4}\le0.
\end{align*}
Fix $\w_{4}\le0$, we have
\begin{align*}
\min_{\d,\boldsymbol{\w}} & \ \left[\frac{1}{1-\w_{4}}\beta^{2}/\gamma^{2}+\frac{1}{1-\w_{4}}-2\frac{\w_{4}}{\w_{4}-1}\beta/\gamma\right]\w_{4}\gamma^{2}\\
\text{s.t.} & \ (1-\w_{4})\alpha+\left(\beta+\gamma\right)\w_{4}=0\\
 & \ \left|\alpha\right|,\left|\beta\right|,\left|\gamma\right|\le1\\
 & \ \frac{1-c}{2}\le\w_{4}\le0.
\end{align*}
Here we suppose that $\gamma^{2}\ge\beta^{2}$ and $\gamma^{2}\ge\alpha^{2}$
and it is obvious that $\gamma=1$ (or -1, which is the same). We
reduce the problem to

\begin{align*}
\min_{\d,\boldsymbol{\w}} & \ \left[\frac{1}{1-\w_{4}}\beta^{2}+\frac{1}{1-\w_{4}}-2\frac{\w_{4}}{\w_{4}-1}\beta\right]\w_{4}\\
\text{s.t.} & \ (1-\w_{4})\alpha+\left(\beta+1\right)\w_{4}=0\\
 & \ \left|\alpha\right|,\left|\beta\right|\le1\\
 & \ \frac{1-c}{2}\le\w_{4}\le0.
\end{align*}
And in this case, it is obvious that $\beta=-1$, which gives that
$\alpha=0$ and thus the problem reduce to binary case.

\paragraph{Case 1 $\protect\w_{1}\ge0$, $\protect\w_{2}\ge0$, $\protect\w_{3}\le0$}

Case 2 has the same argument by setting $\w_{4}=\w_{1}+\w_{2}$.
\fi 
